# Supplementary material for: Ultrafast X-ray imaging of pulsed plasmas in water
Source: arXiv:2007.14631 source file (2020-07-29)
Supplement: Supplementary file 1 [file SM.pdf]

# Supplementary Material: Ultrafast X-ray imaging of pulsed plasmas in water

Christopher Campbell,[1] Xin Tang,[1] Yancey Sechrest,[2] Kamel Fezzaa,[3] Zhehui Wang,[2] and David Staack[1]
[1]*Department of Mechanical Engineering, Texas A&M University, College Station, TX 77843, USA*
[2]*Los Alamos National Laboratory, Los Alamos, NM 87545, USA*
[3]*X-ray Science Division, Advanced Photon Source, Argonne National Laboratory, Argonne, IL 60439, USA.*
(Dated: July 28, 2020)

## I. EXPERIMENTAL SETUPS USED IN THIS WORK

The results presented in this work used two separate plasma imaging setups to interrogate the pulsed water plasma of interest. In each case, the plasma circuit consisted of a Spellman SL300 supply powering a high-voltage RC charging circuit (see Figure 2a), which in turn powered an air spark gap in series with the water plasma discharge of interest to this work. Nanosecond electrical diagnosis was achieved using a 500-MHz Tektronix DPO3054 oscilloscope, Northstar PVM-4 voltage probe, and Bergoz CT-D1.0 current probe. From simultaneous voltage and current measurement (Figure 2b), instantaneous power and energy was calculated from $E(t) = \int_0^t P(t')dt' = \int_0^t V(t')I(t')dt'$ (Figure 2c). To facilitate time-resolved diagnostics, the circuit uses an Nd:YAG high-power laser (Gemini PIV, by New Wave Research) to trigger the air spark gap switch in series with the water discharge cell, resulting in the low-jitter event timing (~10ns) needed for time-resolved imaging techniques. To image the plasma of interest, an imaging train can be assembled oriented normal to the water cell window visible in Figure 2a. Optical imaging presented in this work was done using both a Photron SA-5 CMOS video camera (Figure 3a) and a 4Picos ICCD from Stanford Computer Optics (Figure 3b), in conjunction with a fixed-focus microscope lens.

For phase-contrast X-ray, the APS 32-ID-B beamline experimental setup shown in Figure SM1 was used, which employs the imaging configuration shown in Figure SM2. Our X-ray imaging campaign used singlets (50ps RMS duration, 120 FWHM) provided by a hybrid pulse train from the APS, which were spaced by 3.68 µs; 272-kfps (every singlet) and 136-kfps (every other singlet) modes were used. A Photron SA-Z high speed camera was used in conjunction with a LuAG scintillator to image the X-ray singlets.

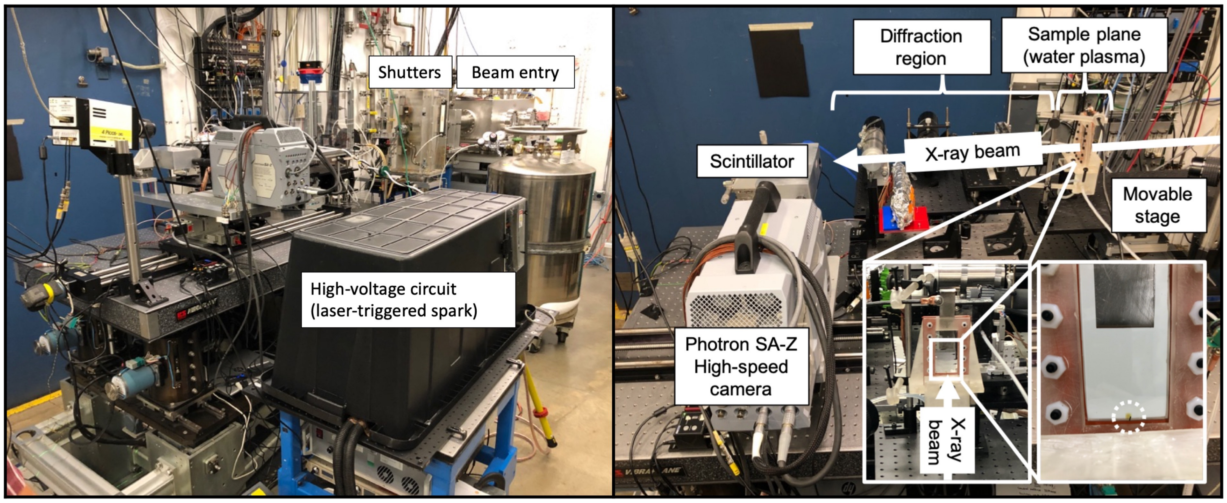


FIG. SM1. Water corona X-ray imaging experimental setup in the APS 32-ID-B beamline experiment hutch. The dashed circle (inset, right) outlines the approximate field of view used for X-ray imaging. The laser-triggered air spark pulsing circuit which generated the plasma of interest to the X-ray diagnostic is described in Figure SM2.

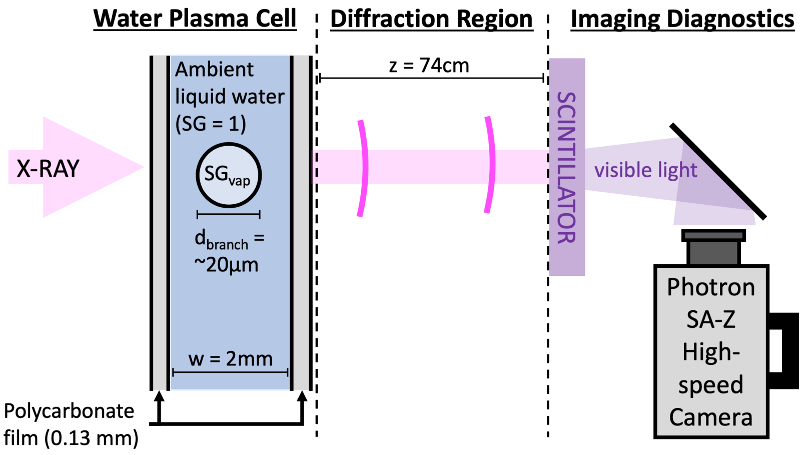


FIG. SM2. Schematic of the phase-contrast X-ray imaging setup used in this work at the APS 32-ID-B beamline lab. The environment within the water plasma cell shows the cross-section of a typical cylindrical plasma channel, which serves as the assumed geometry for the computational model.

## II. MULTI-FRAME X-RAY IMAGING OF SELECTED WATER CORONA DISCHARGE EVENTS

Over the course of this experimental campaign at APS, a total of 107 plasma events were imaged in X-ray. Of these, we present here multi-frame imaging of five selected typical events (Figures SM3–SM7), with each frame timestamped relative to the instant of plasma initiation (peak current). In each of these events, note the evolution from the pre-event environment to small-diameter long plasma channels, and then to large-diameter cavitation and expansion.

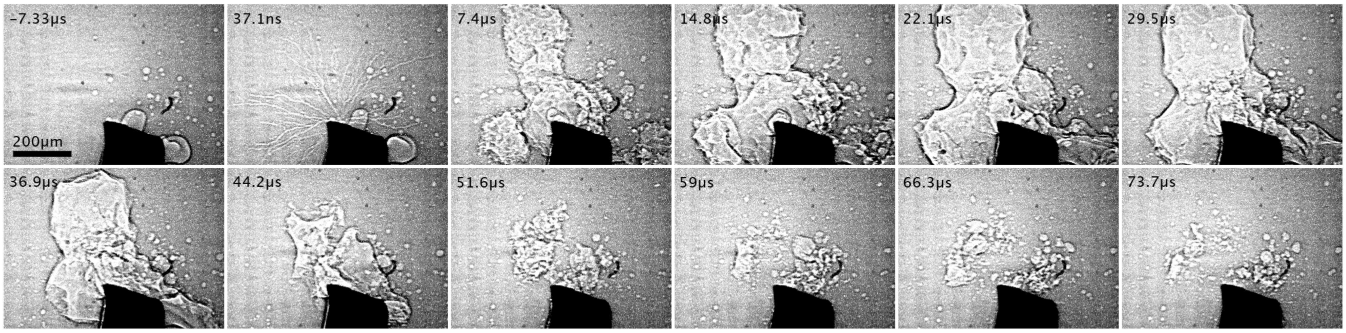


FIG. SM3. X-ray framerate of 136 kfps (7.37 µs/frame).

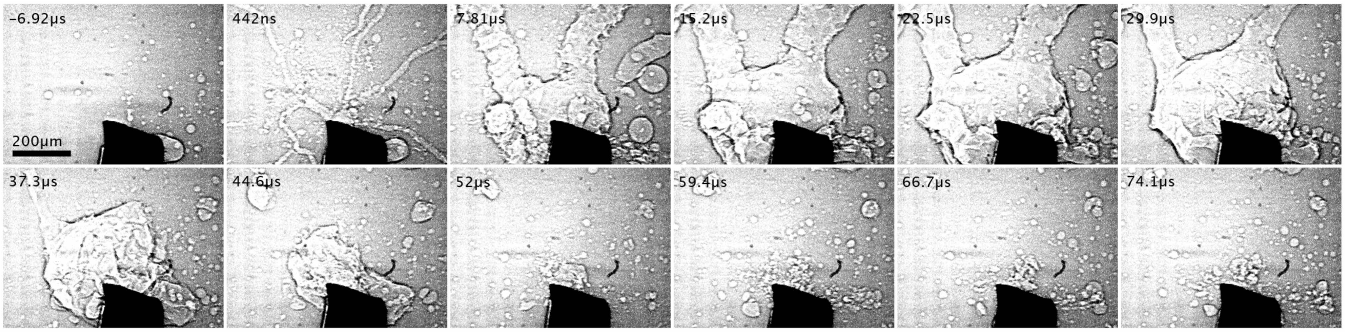


FIG. SM4. X-ray framerate of 136 kfps (7.37 µs/frame).

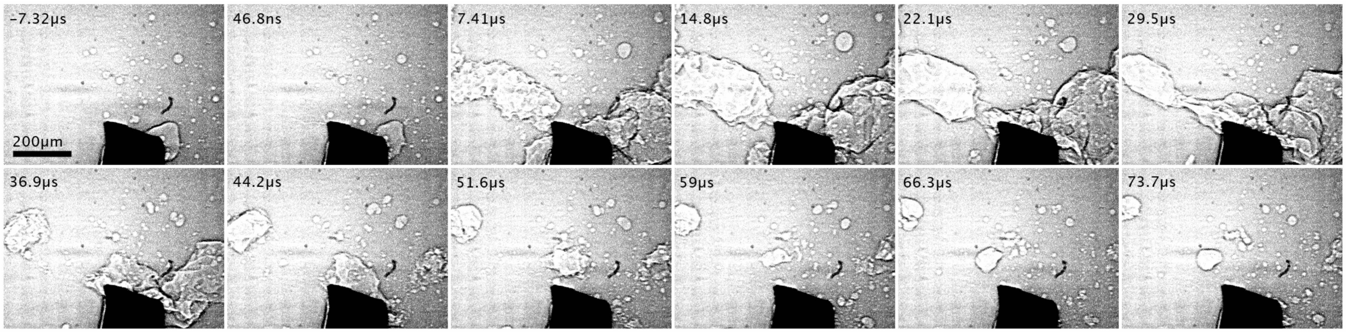


FIG. SM5. X-ray framerate of 136 kfps (7.37 μs/frame).

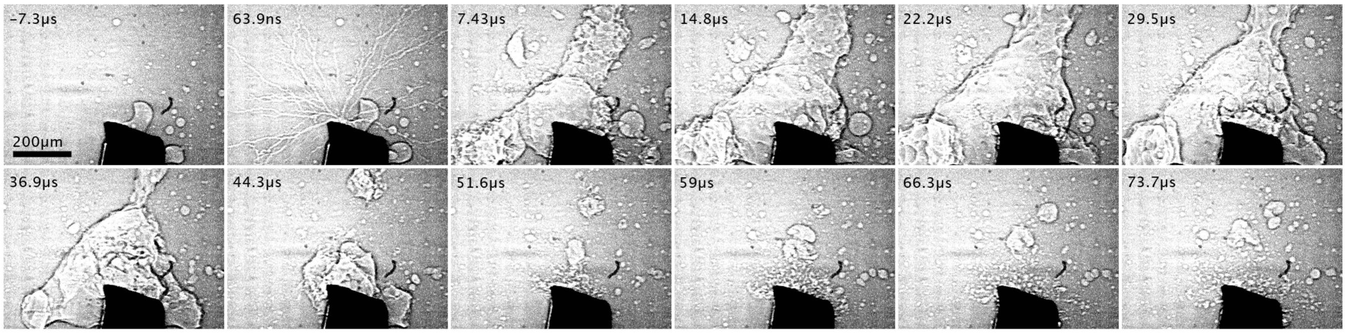


FIG. SM6. X-ray framerate of 136 kfps (7.37 μs/frame).

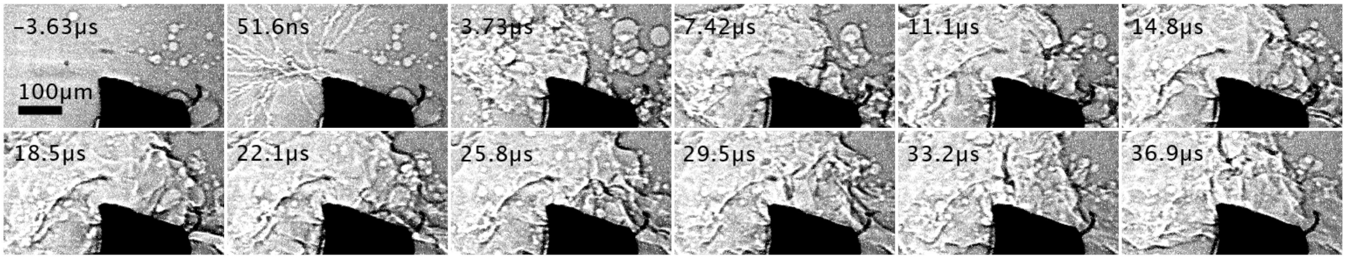


FIG. SM7. X-ray framerate of 272 kfps (3.69 μs/frame).

## III. SMALL-ANGLE DIFFRACTION INTEGRAL FOR PHASE-CONTRAST IMAGING OF CYLINDRICAL BUBBLES: ANALYTICAL DERIVATION AND UNCERTAINTY ANALYSIS

The general form of the diffraction integral for two-dimensional sample and detector planes seperated by a distance $z$ can be expressed as follows:

$$g_{\text{out}}(x',y') = \frac{e^{2\pi iz/\lambda}}{i\lambda z}\int_{-\infty}^{\infty}\int_{-\infty}^{\infty} g_{\text{in}}(x,y)e^{\frac{i\pi}{\lambda z}\left((x'-x)^2+(y'-y)^2\right)}dxdy \tag{1}$$

where and $(x,y)$ and $(x',y')$ are positions on the sample and detector planes, respectively. The terms $g_{\text{in}}$ and $g_{\text{out}}$ represent electric field before and after the diffraction region. The paraxial approximation $\sqrt{(x'-x)^2+(y'-y)^2} \ll z$ has been applied, and $z = 74$ cm for the results presented in this work. For cylindrical samples oriented perpendicular to the optical axis, symmetry implies $g_{\text{in}}(x,y) = g_{\text{in}}(x)$ and $g_{\text{out}}(x',y') = g_{\text{out}}(x')$, enabling evaluation of the $y$-integral:

$$\begin{aligned} g_{\text{out}}(x') &= \frac{e^{2\pi iz/\lambda}}{i\lambda z}\int_{-\infty}^{\infty}\int_{-\infty}^{\infty} g_{\text{in}}(x)e^{\frac{i\pi}{\lambda z}\left((x'-x)^2+(y'-y)^2\right)}dxdy && (2)\\ &= \frac{e^{2\pi iz/\lambda}}{i\lambda z}\int_{-\infty}^{\infty} g_{\text{in}}(x)e^{\frac{i\pi}{\lambda z}(x'-x)^2}dx\int_{-\infty}^{\infty} e^{\frac{i\pi}{\lambda z}(y'-y)^2}dy && (3)\\ &= \frac{e^{2\pi iz/\lambda}}{\sqrt{i\lambda z}}\int_{-\infty}^{\infty} g_{\text{in}}(x)e^{\frac{i\pi}{\lambda z}(x'-x)^2}dx && (4) \end{aligned}$$

The function $g_{\text{in}}(x)$ completely describes the sample plane and must be defined explicitly. We assume the pre-sample X-ray beam to be coherent, collimated, and in phase. If we normalize by $g_{\text{beam}}$, the post-sample beam electric field $g_{\text{in}}$ can be expressed via $g_{\text{in}}(x) = g_{\text{beam}}(x)g_t(x) = g_t(x)$ where $g_t(x)$ is the following piecewise function:

$$g_t(x) = \begin{cases} e^{\left[\frac{-2i\pi}{\lambda}\tilde{n}_{\text{water,liq}}\cdot w_{\text{liq}}\right]}, & |x| > R \\ e^{\left[\frac{-2i\pi}{\lambda}\tilde{n}_{\text{water,liq}}\cdot(w_{\text{liq}}-2\sqrt{R^2-x^2})\right]}\cdot e^{\left[\frac{-2i\pi}{\lambda}\tilde{n}_{\text{water,vap}}\cdot(2\sqrt{R^2-x^2})\right]}, & |x| \le R \end{cases} \tag{5}$$

where $\tilde{n} = 1-\delta-i\beta$ is the complex index of refraction of a given medium, $R$ is the radius of the cylindrical bubble, $w_{\text{liq}}$ is the thickness of the water cell (∼2mm in this work), and $x = 0$ is the centerline of the bubble. This defines a computational domain matching the geometry shown in Figure SM2. The windows of the cell are made of 0.005" polycarbonate plastic which attenuates ∼0.5% of the beam, and may be neglected for the purposes of this work. The indices of refraction for ambient water and for a low-density water vapor region of specific gravity $SG_{\text{vap}}$ are related via $\delta_{\text{water,vap}} = SG_{\text{vap}}\delta_{\text{water,liq}}$ and $\beta_{\text{water,vap}} = SG_{\text{vap}}\beta_{\text{water,liq}}$. Equation 4 is now fully constrained for a given $R$ and $SG_{\text{vap}}$. By minimizing the error between results from this model and from experiment, we can determine realistic values of $R$ and $SG_{\text{vap}}$. See Figure SM8 as well as Figures 5c and 5d for summary plots of this computational campaign. In addition to $R$ and $SG_{\text{vap}}$, it is necessary to include a few more parameters in the optimization process: relative shifting, relative scaling, and the linear slope of the experimental cutline background. These three additional parameters are not strongly coupled to the primary parameters of interest $R$ and $SG_{\text{vap}}$, however their inclusion is important for successful fitting. See the contour plot in Figure SM9 of the optimization metric (average p-value) as a function of $d_{\text{branch}} = 2R$ and $SG_{\text{vap}}$, which serves as an uncertainty analysis for the result presented in Figure 5.

## IV. SUPPLEMENTARY VIDEOS

Supplementary Video 1 is a complete visible light high-speed video corresponding to the frame-by-frame images shown in Figure 3a. Supplementary Video 2 is a constructed video of 202 sorted ICCD images, a subset of which is shown in Figure 3b. Supplementary Video 3 is a complete X-ray high-speed video corresponding to the frames shown in Figure 4a.

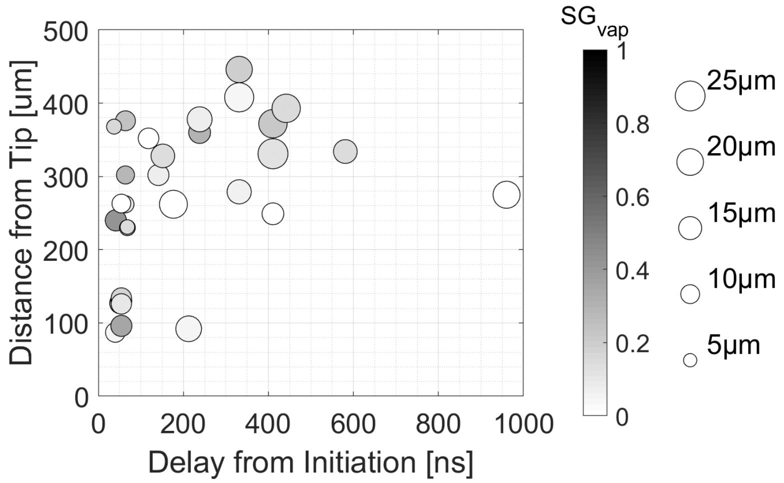


FIG. SM8. Scatter plot results from 31 different model fits, for a variety of different delays relative to peak current and distances from the electrode tip. Point size is proportional to plasma channel diameter $d_{\mathrm{channel}} = 2R$, and point shading represents $SG_{\mathrm{vap}}$. It should be emphasized that point locations in this plot depend on which X-ray images were conducive to cutline interpolation and not on any underlying physical trend. This plot serves as an overall summary of successful model fits, and its constituent data has been recast to generate Figures 5c and 5d.

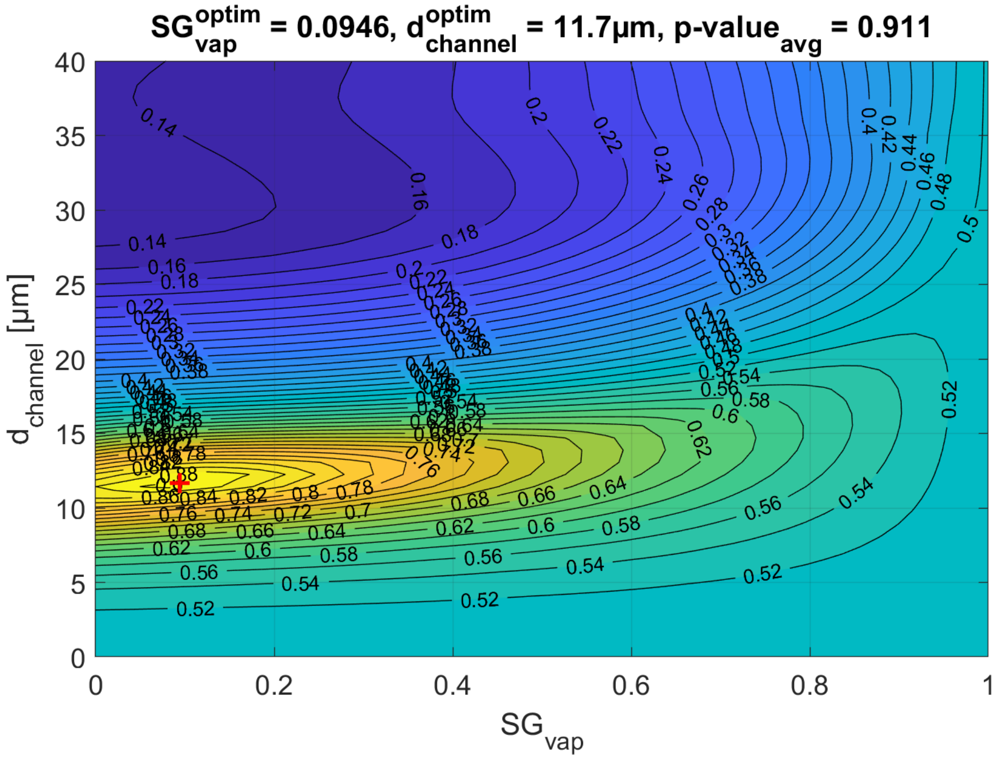


FIG. SM9. Contour plot of optimization metric (average p-value) as a function of $d_{\mathrm{branch}}$ and $SG_{\mathrm{vap}}$, for the result presented in Figure 5 of the main text. Uncertainty can be defined by the contour line at 90% of the optimized value, which in this case is at a p-value of 0.82. We therefore interpret this result as $d_{\mathrm{branch}} = 11.7^{+1.5}_{-1.3}$ μm and $SG_{\mathrm{vap}} = 0.09^{+0.17}_{-0.09}$.
